# Supplementary material for: Cosmic Dragons: A Two-Component Mixture Model of COSMOS Galaxies
Source: arXiv:2310.09374 source file (2024-03-28)
Supplement: Supplementary file 1 [file nix_7Dv3D.tex]

\iffalse
%  %  %  %  %  %  %  %  %  %  %  %  %  %  %  %
\subsection{Difference in selection between extended photometry and DES main bands} \label{sec:7D_vs_3D} 
% Slxn acc for 3D vs 7D

The difference in selection between dragons trained on DES main bands $griz$ and dragons trained on the extended photometry $ugriz + JHK_{\rm s}$ raises the question of mutual compatibility: To what accuracy can a dragon trained on $griz$ bands alone select RS galaxies as defined by a dragon trained on the extended photometry?

\wm{TODO: plot bACC(z) for the three bins, with 7D as `truth'.} 

\begin{figure}\centering
  \includegraphics [width=\linewidth] {figs/bACC_7D_3D}
  \caption[bACC of DES main bands vs extended photometry]{
    Selection accuracy of using DES main bands ($griz$) alone, as compared to the extended photometry sample ($ugriz + JHK_{\rm s}$). 
    \textcolor{red}{[currently only for middle mass bin; preliminary placeholder result.]} 
    Looks like it's roughly 90\% except near the transition redshifts. 
  }
  \label{fig:7D_vs_3D}
\end{figure}

Note: bACC between bootstrap runs is typically $(97 \pm 1)\%$, so that's an effective maximum expected bACC here. Can't really expect bACC to be $\gtrsim 95\%$ when that's only barely the case between bootstraps. 
\fi
